# Supplementary material for: Effects of Strain Compensation on Electron Mobilities in InAs Quantum Wells Grown on InP(001)
Source: arXiv:2406.19469 ancillary file (2025-03-17)
Supplement: Supplementary file 1 [file Effects_of_Strain_Compensation_SI_v3.pdf]

**Effects of Strain Compensation on Electron Mobilities in InAs Quantum Wells Grown on InP(001)**

Connor P. Dempsey[1], Jason T. Dong[2], Irene Villar Rodriguez[3], Yilmaz Gul[3], Shirshendu Chatterjee[1], Mihir Pendharkar[1], Stuart N. Holmes[4], Michael Pepper[3,4], and Christopher J. Palmstrøm[1,2]

[1]Deparment of Electrical and Computer Engineering, University of California, Santa Barbara, CA 93106

[2]Materials Department, University of California, Santa Barbara, CA 93106

[3]London Centre for Nanotechnology, University College London, 17-19 Gordon Street, London WC1H 0AH, United Kingdom

[4]Department of Electronic and Electrical Engineering, University College London, Torrington Place, London WC1E 7JE, United Kingdom

**S1: Depiction of strain within the QW active region**

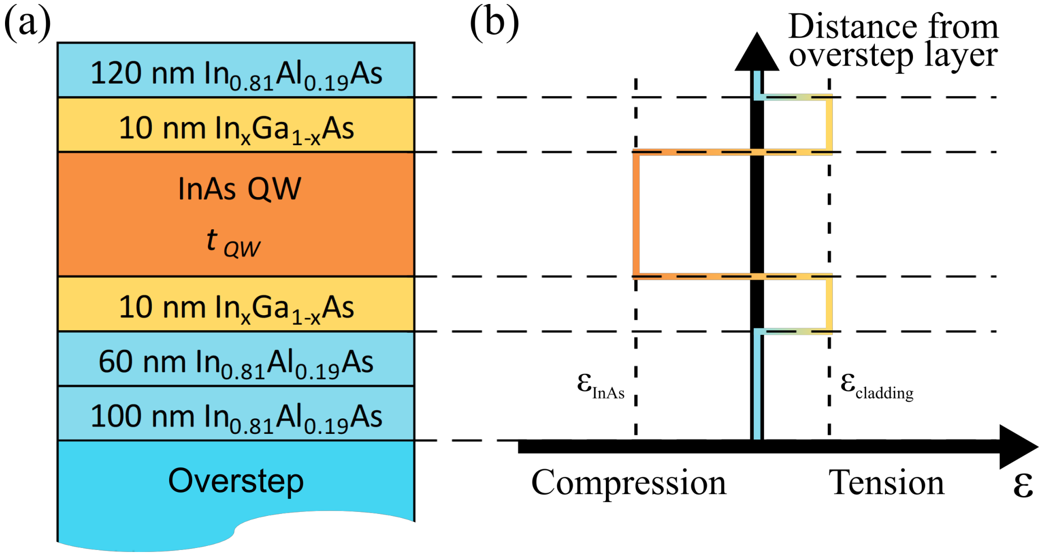


Figure S1: (a) Schematic of the InAs QW active region from the overstep $In_{0.83}Al_{0.17}As$ layer to the top barrier layer of the QW. (b) Representation of the total strain in the active region as a function of the distance from the overstep layer.

The active region of the InAs QW structure is depicted in Fig. S1(a). Key layer transitions are extended into Fig. S1(b) to exhibit the accumulation of strain within the structure as a function of distance from the overstep layer. The smaller lattice constant of the $In_xGa_{1-x}As$ region relative to the $In_{0.81}Al_{0.19}As$ region causes the cladding layers on both sides of the QW to reside in tensile strain, $\varepsilon_{cladding}$, as depicted. The value of $\varepsilon_{cladding}$ is dependent upon the In concentration in the $In_xGa_{1-x}As$ and values of the misfit for compositions with x=0.70, 0.72, 0.74, or 0.81 can be found in Table 1 of the main text. The larger lattice constant of the InAs layer relative to the $In_{0.81}Al_{0.19}As$ barrier causes the QW region to be compressively strained, $\varepsilon_{InAs}$=-1.2%. This counteracts the tensile strain energy accumulated by the cladding regions.

**S2: Measured carrier densities of van der Pauw samples**

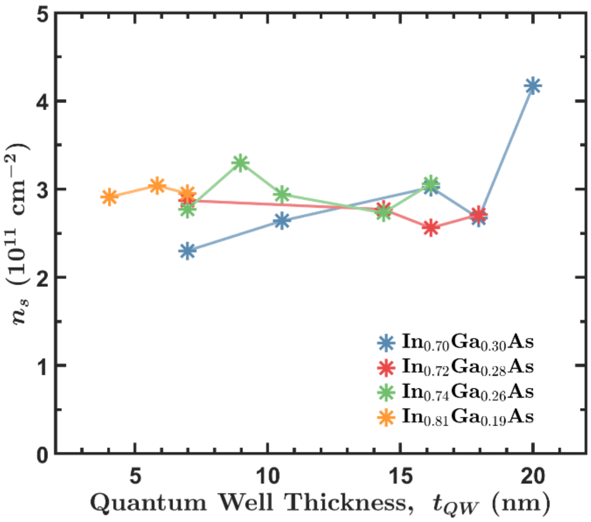


Figure S2: van der Pauw carrier densities extracted from the different $In_xGa_{1-x}As$ concentration series depicted in Fig. 1(b).

The carrier density remains relatively consistent for most of the samples depicted in Fig. 1(b) in the paper. The primarily outlier is the $In_{0.7}Ga_{0.3}As$ sample, which was found to have the highest carrier density recorded of $4.2\times10^{11}$ cm$^{-2}$.

**S3: Calculated Bandgaps for Multiple $t_{QW}$ thicknesses and varying $In_xGa_{1-x}As$ Concentrations**

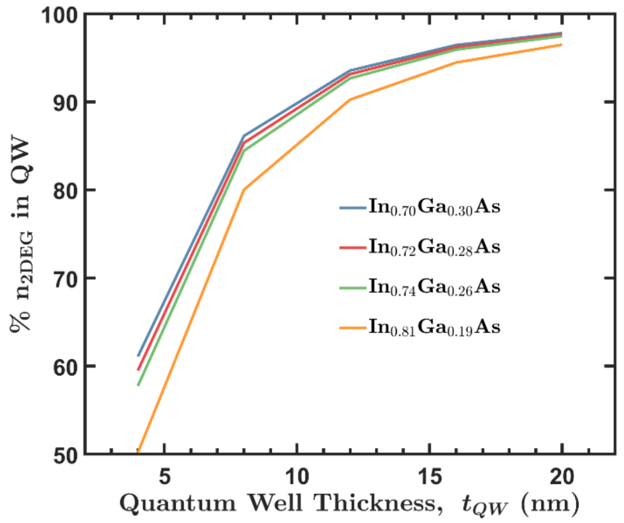


Figure S3: Schrödinger-Poisson calculation [1] of the percentage of 2DEG state contained within QW for various thicknesses and $In_xGa_{1-x}As$ concentrations.

By increasing the Ga concentration in the $In_xGa_{1-x}As$ layer, the band gap of the cladding layer increases. This leads to an increase in the percentage of the 2DEG state that resides within the QW, as depicted in Fig. S3. In all cases, the percentage of the QW is higher for simulations with higher Ga-concentration cladding layers. Additionally, the simulation demonstrates the relationship between the thickness of the QW and the percentage of carriers residing within the well. Clearly, by increasing the QW thickness the percentage of the 2DEG residing within the well can be increased.

**S4: Extended top gate measurements on $In_{0.72}Ga_{0.28}As$ QW**

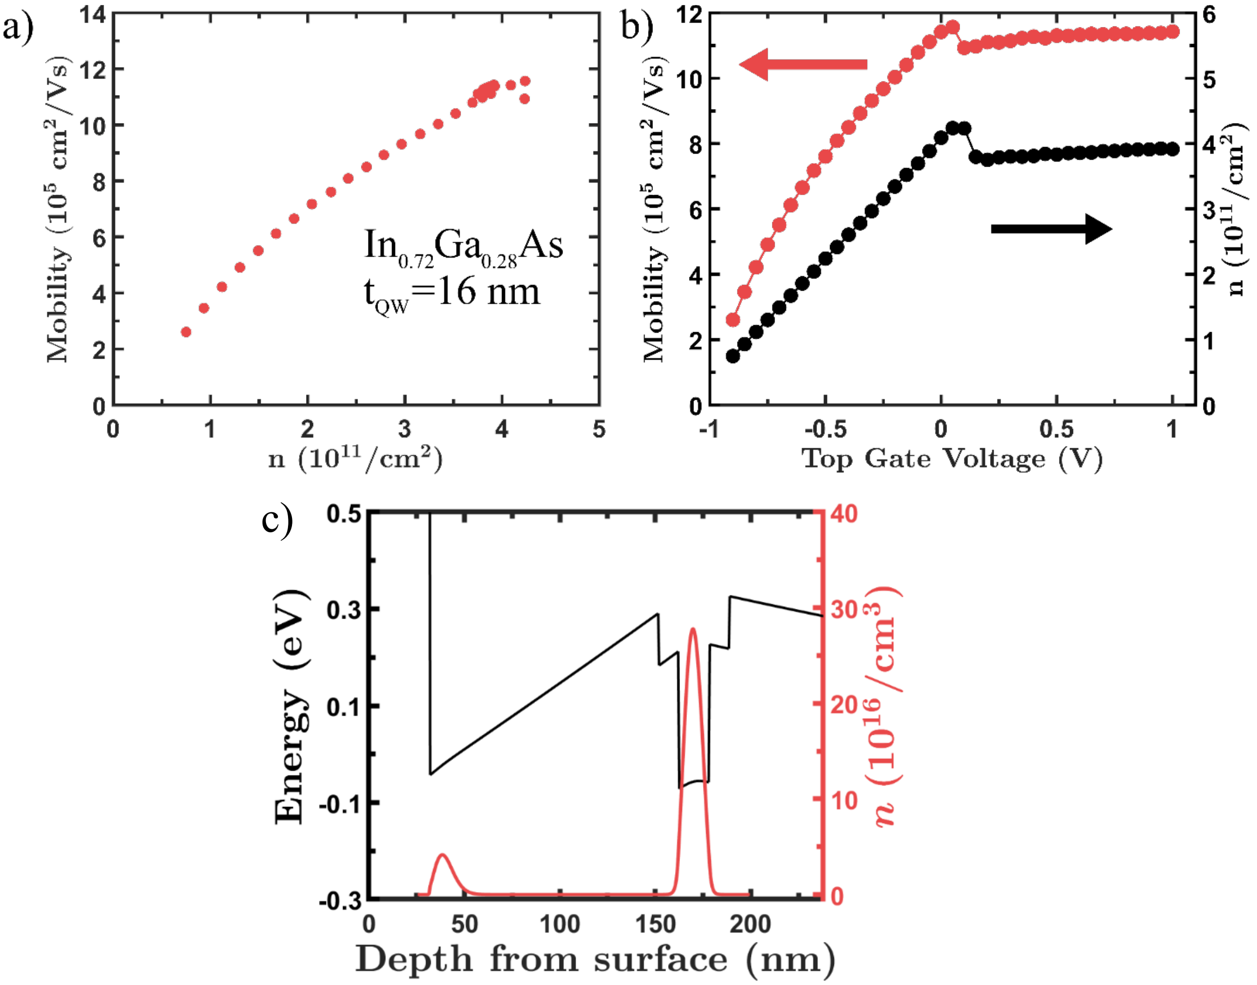


Figure S4: a) Mobility vs. carrier density for the 16 nm thick InAs QW with $In_{0.72}Ga_{0.28}As$ cladding layers. b) Relationship of mobility (left) and carrier density (right) compared to the applied top gate voltage. c) Schrödinger-Poisson simulation [1] of an applied top gate voltage (+0.2V) on the 16 nm thick $In_{0.72}Ga_{0.28}As$ QW.

Fig. S4(a) depicts a the mobility and carrier density relationship for a wider range of applied top gate voltages than depicted in Fig. 3(a). This wider range shows a cluster of points near $3.8\times10^{11}$ $cm^{-2}$, which does not appear for limited top gate voltages. To better understand this clustering of points, the relationship of mobility and carrier density were plotted against the top gate voltage, as depicted in Fig. S4(b). As the top gate voltage is increased beyond +0.05V, where the maximum achieved mobility of $1.16\times10^6$ $cm^2/Vs$ occurs, the mobility drops. This is not unexpected and typically indicates that the second subband of the QW has begun to fill [2,3,4] because the increase in the available number of states leads to an increase in the overall scattering rate and thereby a drop in the total mobility. Surprisingly, beyond +0.05V, the carrier density also drops and filling of the QW continues but at a much lower rate relative to the increase in top gate voltage. One potential explanation for this observation is the formation and filling of an unintentional 2DEG state formed at the interface between the $AlO_x$ dielectric and the $In_{0.81}Al_{0.19}As$ barrier layers, as depicted in Fig. S4(c). At low top gate voltages, an interfacial 2DEG state would be fully

depleted and all of the carriers would reside in the QW. As the top gate voltage increases, the interfacial 2DEG will eventually begin to fill, potentially pulling carriers away from the 2DEG and screening the QW from further increases in the applied top gate voltage.

**S5: Reciprocal space maps of 16 nm InAs QW with $In_{0.72}Ga_{0.28}As$ cladding layers**

a)

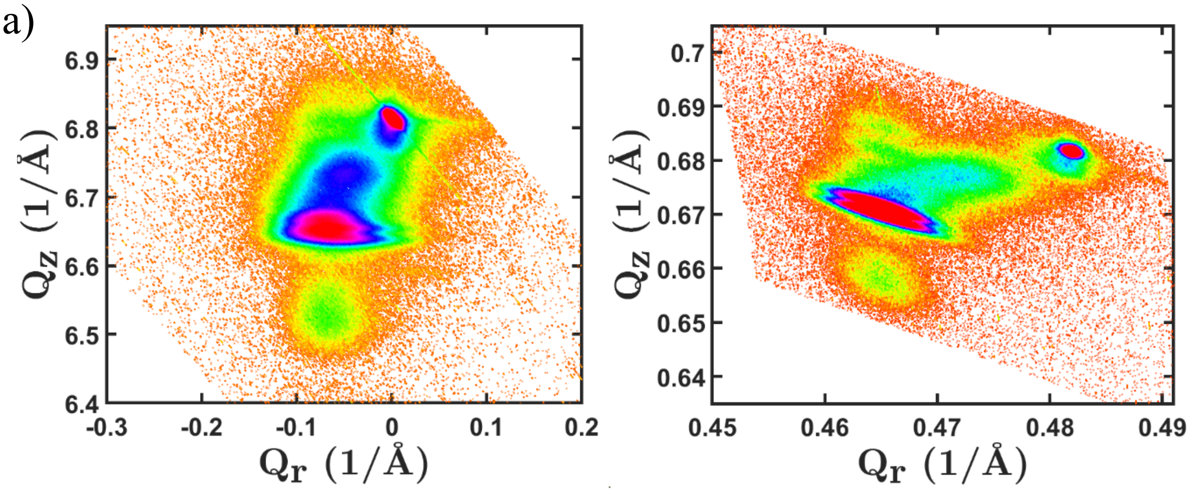


Figure S5: a) Reciprocal space map (RSM) of (004) diffraction peak of the 16 nm thick InAs QW (Sample B) with $In_{0.72}Ga_{0.28}As$ cladding layers. Shift of the QW layers away from $Q_r$=0 $Å^{-1}$ indicate an accumulation of tilt in the buffer layer structure. b) RSM of the $(\bar{2}24)$ diffraction peak showing the appearance of superlattice fringes.

Fig. S5(a) depicts the reciprocal space map of the (004) reflection for the 16 nm thick InAs QW (Sample B) with $In_{0.72}Ga_{0.28}As$ cladding layers. The shift of the location of the InAs QW peak, the $In_{0.72}Ga_{0.28}As$ cladding layers, and the $In_xAl_{1-x}As$ barrier and step graded buffer layers away from $Q_r$=0 indicate that during the relaxation process, the film accumulates a tilt of nearly 0.6° relative to the substrate. Fig. S5(b) depicts the reciprocal space map of the $(\bar{2}24)$ reflection for the same QW. Superlattice fringes can be observed more clearly in this figure. While surprising given the lack of periodic structures with a similar in-plane lattice constant to the $In_{0.81}Al_{0.19}As$ layers, superlattice reflections have been observed in both simulations and measurements of previous QW samples despite the absence of a periodic structure [5].

**S6: Additional data showing temperature dependence of Rashba response**

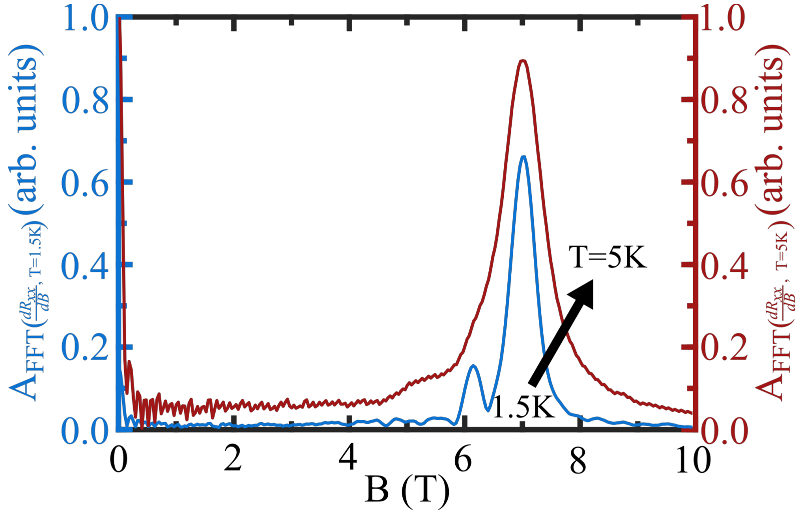


Figure S6: *Left axis:* FFT of the $dR_{xx}/dB$ spectrum taken at 1.5K, as shown in Fig. 5(b) of the main text, depicting two Rashba split peaks. *Right axis:* FFT of the $dR_{xx}/dB$ spectrum taken at 5K, demonstrating that the secondary peak disappears with increasing temperature.

As discussed in the main text, the modulated magnetic field technique enables a highly sensitive and direct measurement of the first and second derivatives of the longitudinal resistance, $R_{xx}$. The blue plot and left axis of Fig S6 depicts the FFT of $dR_{xx}/dB$, as depicted in Fig. 5(b) of the main text. At a sample temperature of 1.5 K, a clear secondary peak can be observed in the spectra. Secondary peaks in the FFT spectrum can also occur due to magneto-intersubband scattering (MIS) or magnetophonon resonance (MPR) effects. To determine whether or not the secondary peak occurs due to either of these effects, the sample temperature was increased to 5K. The modulated magnetic field measurement was repeated and the resulting FFT is depicted in red and on the right axis of Fig. S6. At 5K, the Rashba split peak has disappeared. Given the typical temperature insensitivity of both MIS and MPR [6], and the highly temperature sensitive nature of the secondary peak, it is unlikely that the secondary peak is caused by either of these two effects.

**Bibliography:**

[1] Tan, I.-H., Snider, G. L., Chang, L. D., & Hu, E. L. (1990). A self-consistent solution of Schrödinger–Poisson equations using a nonuniform mesh. *J. Appl. Phys.*, *68*(8), 4071–4076.

[2] Hatke, A. T., Wang, T., Thomas, C., Gardner, G. C., & Manfra, M. J. (2017). Mobility in excess of $10^6$ $cm^2/Vs$ in InAs quantum wells grown on lattice mismatched InP substrates. *Applied Physics Letters*, *111*(14), 142106.

[3] Thomas, C., Hatke, A. T., Tuaz, A., Kallaher, R., Wu, T., Wang, T., Diaz, R. E., Gardner, G. C., Capano, M. A., & Manfra, M. J. (2018). High-mobility InAs 2DEGs on GaSb substrates: A platform for mesoscopic quantum transport. *Physical Review Materials*, *2*(10), 104602.

[4] Tschirky, T., Mueller, S., Lehner, C. A., Fält, S., Ihn, T., Ensslin, K., & Wegscheider, W. (2017). Scattering mechanisms of highest-mobility InAs/$Al_xGa_{1-x}Sb$ quantum wells. *Physical Review B*, *95*(11), 115304.

[5] Nguyen, B. M., Yi, W., Noah, R., Thorp, J., & Sokolich, M. (2015). High mobility back-gated InAs/GaSb double quantum well grown on GaSb substrate. *Applied Physics Letters*, *106*(03), 032107.

[6] Osako, S., Hamano, T., Mori, N., Hamaguchi, C., Sasa, S., & Inoue, M. (1998). Magnetophonon and magneto-intersubband-scattering effects in InAs/AlGaSb heterostructures. *Physica B*, *249–251*, 740–744.
